# Supplementary material for: When does Subgroup Balance Matter? Predicting Performance Sensitivity from Latent Separability
Source: arXiv:2512.09496 source file (2026-10-20)
Supplement: Supplementary file 1 [file dataset_details_table.tex]

\begin{table}[h]
\caption{Details on the datasets used for mitigation experiments.}
\label{tab: dataset details}
\begin{small}
\begin{center}
\begin{tabular}{lllll}
\toprule
\textbf{Dataset}      & \textbf{MNIST}    & \textbf{CheXPert}       & \textbf{CelebA}  & \textbf{Civil\_comments} \\ \midrule
\textbf{Y}            & Even/odd digit    & Pleural effusion        & Blonde hair      & Toxicity                 \\ 
\textbf{A}            & Background colour & Presence of a pacemaker & Perceived gender & Gender                   \\ 
\textbf{S}            & Foreground colour & Sex                     & Smiling          & Religion                 \\ 
\textbf{Dataset size} & 60000              & 3225                    & 12500            & 8900                     \\ \bottomrule
\end{tabular}
\end{center}
\end{small}
\end{table}
